# Supplementary material for: The main asteroid belt: the primary source of debris on comet-like orbits
Source: arXiv:2105.07442 source file (2021-05-16)
Supplement: Supplementary file 1 [file appendix_table.pdf]

# Table A1

| event_codename | percent_unstable_10kyrs | stdev_percent_unstable_10kyrs | datetime | jd | sol_long | duration | num_datapoints | slope | initial_slope_err | best_convergence_angle | initial_latitude |
|---|---|---|---|---|---|---|---|---|---|---|---|
| DN140926_01 | 28.3 | 3.1 | 2014-09-26T16:4 | 2456927.197 | 183.32 | 8.14 | 448 | 13.67 | 0.01 | 89.70 | -29.07578 |
| DN141213_01 | 0 | 0.0 | 2014-12-13T13:3 | 2457005.063 | 261.25 | 1.2 | 90 | 31.19 | 0.02 | 87.98 | -30.63355 |
| DN150112_01 | 17.1 | 3.7 | 2015-01-12T13:1 | 2457035.052 | 291.79 | 1.16 | 31 | 57.50 | 0.01 | 13.44 | -30.42794 |
| DN150311_02 | 0 | 0.0 | 2015-03-11T17:4 | 2457093.236 | 350.61 | 1.06 | 42 | 63.86 | 0.01 | 22.72 | -28.83280 |
| DN150324_01 | 10.3 | 2.8 | 2015-03-24T19:4 | 2457106.322 | 3.64 | 3.118 | 150 | 33.00 | 0.01 | 51.91 | -29.55919 |
| DN150324_02 | 0 | 0.0 | 2015-03-24T19:3 | 2457106.315 | 3.63 | 2.2 | 81 | 40.14 | 0.01 | 49.40 | -27.27782 |
| DN150328_01 | 0 | 0.0 | 2015-03-28T18:2 | 2457110.268 | 7.55 | 0.76 | 30 | 76.74 | 0.01 | 86.35 | -28.41105 |
| DN150411_01 | 0 | 0.0 | 2015-04-11T16:4 | 2457124.196 | 21.26 | 1.02 | 28 | 70.03 | 0.01 | 43.64 | -29.52816 |
| DN150420_01 | 5.9 | 2.8 | 2015-04-20T15:4 | 2457133.159 | 30.04 | 1.12 | 42 | 75.37 | 0.01 | 41.79 | -32.06586 |
| DN150712_03 | 4.7 | 1.2 | 2015-07-12T11:3 | 2457215.981 | 109.61 | 1.96 | 77 | 55.14 | 0.01 | 35.77 | -29.72626 |
| DN150714_05 | 0 | 0.0 | 2015-07-14T19:4 | 2457218.32 | 111.84 | 2.06 | 78 | 44.40 | 0.00 | 35.55 | -30.20574 |
| DN150816_01 | 49.8 | 5.6 | 2015-08-16T18:4 | 2457251.282 | 143.38 | 3.22 | 154 | 31.58 | 0.01 | 30.94 | -29.53794 |
| DN150816_03 | 13.6 | 2.7 | 2015-08-16T18:2 | 2457251.265 | 143.36 | 1.16 | 44 | 45.99 | 0.01 | 44.15 | -32.17261 |
| DN150816_04 | 83.6 | 4.0 | 2015-08-16T18:4 | 2457251.282 | 143.38 | 3.02 | 104 | 31.15 | 0.01 | 30.96 | -29.53529 |
| DN150817_01 | 86.1 | 5.5 | 2015-08-17T12:3 | 2457252.025 | 144.09 | 2.86 | 118 | 57.48 | 0.00 | 44.29 | -29.92115 |
| DN150905_01 | 0 | 0.0 | 2015-09-05T14:1 | 2457271.09 | 162.49 | 4.36 | 211 | 44.98 | 0.01 | 37.75 | -30.51809 |
| DN150909_03 | 0 | 0.0 | 2015-09-09T17:4 | 2457275.241 | 166.52 | 1.26 | 51 | 56.03 | 0.02 | 72.84 | -30.62502 |
| DN151021_03 | 0 | 0.0 | 2015-10-21T19:1 | 2457317.3 | 207.85 | 1.791 | 102 | 38.84 | 0.02 | 60.70 | -28.79235 |
| DN151210_01 | 0 | 0.0 | 2015-12-10T17:4 | 2457367.236 | 258.12 | 1.16 | 46 | 64.13 | 0.01 | 87.59 | -31.23286 |
| DN160303_01 | 0 | 0.0 | 2016-03-03T18:4 | 2457451.28 | 343.40 | 1.04 | 44 | 48.84 | 0.01 | 66.00 | -30.98304 |
| DN160409_02 | 0 | 0.0 | 2016-04-09T11:3 | 2457487.979 | 19.82 | 1.32 | 50 | 57.95 | 0.01 | 24.30 | -30.79361 |
| DN160502_01 | 0 | 0.0 | 2016-05-02T13:3 | 2457511.063 | 42.35 | 1.322 | 112 | 62.17 | 0.01 | 86.84 | -31.57716 |
| DN160505_02 | 0 | 0.0 | 2016-05-05T20:0 | 2457514.335 | 45.52 | 2.16 | 114 | 36.40 | 0.02 | 83.12 | -32.86269 |
| DN160507_02 | 0 | 0.0 | 2016-05-07T13:3 | 2457516.069 | 47.20 | 1.42 | 109 | 41.55 | 0.01 | 78.79 | -30.23895 |
| DN160512_01 | 0 | 0.0 | 2016-05-12T18:0 | 2457521.254 | 52.21 | 1.02 | 86 | 71.87 | 0.01 | 81.92 | -29.63938 |
| DN160513_01 | 0 | 0.0 | 2016-05-13T15:0 | 2457522.129 | 53.05 | 1.42 | 126 | 62.80 | 0.01 | 79.83 | -31.47673 |
| DN160517_01 | 0 | 0.0 | 2016-05-17T19:3 | 2457526.314 | 57.09 | 1.16 | 46 | 50.35 | 0.01 | 36.69 | -32.29303 |
| DN160518_03 | 0 | 0.0 | 2016-05-18T18:0 | 2457527.254 | 57.99 | 1.12 | 63 | 62.99 | 0.01 | 84.39 | -29.65052 |
| DN160701_01 | 0 | 0.0 | 2016-07-01T19:3 | 2457571.316 | 100.15 | 0.493 | 20 | 77.43 | 0.01 | 31.00 | -29.38782 |
| DN160721_03 | 31.1 | 4.7 | 2016-07-21T12:1 | 2457591.007 | 118.93 | 2.26 | 123 | 47.77 | 0.01 | 38.66 | -26.40457 |
| DN160724_13 | 0 | 0.0 | 2016-07-24T16:0 | 2457594.171 | 121.95 | 1 | 39 | 70.20 | 0.01 | 36.27 | -32.27057 |
| DN160810_02 | 0 | 0.0 | 2016-08-10T12:5 | 2457611.035 | 138.09 | 1.66 | 101 | 44.58 | 0.01 | 45.18 | -31.62095 |
| DN160818_01 | 0 | 0.0 | 2016-08-18T18:1 | 2457619.259 | 145.99 | 1.72 | 72 | 64.98 | 0.01 | 68.80 | -31.09322 |
| DN160903_02 | 0 | 0.0 | 2016-09-03T12:2 | 2457635.016 | 161.20 | 1.52 | 64 | 33.45 | 0.01 | 37.30 | -31.36731 |
| DN161026_01 | 0 | 0.0 | 2016-10-26T18:2 | 2457688.265 | 213.53 | 0.76 | 31 | 50.96 | 0.01 | 73.85 | -30.20339 |
| DN161028_02 | 90.8 | 3.0 | 2016-10-28T10:4 | 2457689.95 | 215.22 | 2.92 | 467 | 49.90 | 0.02 | 88.95 | -29.07193 |
| DN161107_01 | 0 | 0.0 | 2016-11-07T18:3 | 2457700.274 | 225.56 | 1.124 | 65 | 82.41 | 0.01 | 45.70 | -32.10249 |
| DN161126_01 | 0 | 0.0 | 2016-11-26T18:5 | 2457719.29 | 244.73 | 0.86 | 33 | 67.29 | 0.01 | 83.37 | -30.72520 |
| DN161129_04 | 0 | 0.0 | 2016-11-29T16:4 | 2457722.2 | 247.67 | 1.538 | 216 | 66.18 | 0.03 | 89.65 | -30.58855 |
| DN170426_01 | 0 | 0.0 | 2017-04-26T14:3 | 2457870.111 | 36.31 | 0.96 | 55 | 72.30 | 0.01 | 77.35 | -30.32805 |
| DN170604_01 | 0 | 0.0 | 2017-06-04T12:4 | 2457909.034 | 73.85 | 1.35 | 39 | 70.36 | 0.01 | 55.90 | -31.72421 |
| DN170731_01 | 0 | 0.0 | 2017-07-31T19:1 | 2457966.302 | 128.52 | 1.4 | 52 | 49.59 | 0.01 | 18.20 | -31.46539 |
| DN170825_02 | 0 | 0.0 | 2017-08-25T11:5 | 2457990.997 | 152.24 | 1.56 | 39 | 22.70 | 0.01 | 9.32 | -33.29298 |
| DN180405_03 | 0 | 0.0 | 2018-04-05T12:5 | 2458214.041 | 15.44 | 1.5 | 30 | 34.07 | 0.00 | 65.21 | -28.47304 |
| DN191020_02 | 0 | 0.0 | 2019-10-20T04:0 | 2458776.668 | 206.20 | 4 | 115 | 31.69 | 0.01 | 27.54 | 40.44304 |
| DN191210_01 | 0 | 0.0 | 2019-12-10T20:5 | 2458828.371 | 258.23 | 1.5 | 55 | 62.87 | 0.00 | 59.06 | 26.65735 |
| DN191224_01 | 0 | 0.0 | 2019-12-24T15:1 | 2458842.135 | 272.23 | 2.5 | 72 | 53.85 | 0.01 | 7.15 | -30.12281 |
| DN200330_01 | 0 | 0.0 | 2020-03-30T17:4 | 2458939.24 | 10.21 | 1.997 | 78 | 51.76 | 0.01 | 65.91 | -28.85386 |
| DN200503_04 | 3.3 | 1.5 | 2020-05-03T16:5 | 2458973.203 | 43.43 | 1.55 | 73 | 72.46 | 0.01 | 46.91 | -34.36858 |
| DN200511_02 | 27.8 | 5.0 | 2020-05-11T21:3 | 2458981.399 | 51.36 | 3 | 87 | 17.03 | 0.01 | 35.24 | 50.85934 |

# Table A2

| initial_longitude | final_latitude | final_longitude | RA_g | err_RA_g | Dec_g | err_Dec_g | num_cams_astrometry | num_cams_timing | RA_inf | RA_inf_err | Dec_inf | Dec_inf_err |
|---|---|---|---|---|---|---|---|---|---|---|---|---|
| 135.66655 | -27.85237739 | 135.4735012 | 196.2276882 | 0.08706356801 | -64.12240518 | 0.1083480784 | 5 | 4 | -172.2673662 | 0.04804403646 | -73.8560317 | 0.0129728724 |
| 138.67180 | -30.36118577 | 138.3315157 | 140.8801569 | 0.03035270426 | -49.85383078 | 0.01749334839 | 4 | 4 | 139.3023066 | 0.02969241348 | -50.0672894 | 0.01786944799 |
| 124.87332 | -30.51626944 | 124.7947723 | 94.45963632 | 0.01373598961 | -1.119010465 | 0.02744271154 | 2 | 1 | 93.07584567 | 0.008035176703 | -3.50339781 | 0.008238036859 |
| 130.37780 | -28.96709734 | 130.4602849 | 191.1591526 | 0.009011103822 | -5.058674417 | 0.008164237474 | 2 | 2 | -168.5623427 | 0.008981003755 | -5.585638174 | 0.009977931241 |
| 126.58875 | -29.7377758 | 127.2367669 | 188.601513 | 0.02218573214 | -1.422292932 | 0.01438418322 | 3 | 3 | -169.2728345 | 0.008145693047 | -2.823375707 | 0.008229322385 |
| 139.72622 | -27.43611136 | 140.3178049 | 206.2708341 | 0.01066516874 | -5.131731054 | 0.01020118826 | 2 | 2 | -152.7598421 | 0.009722967745 | -5.707934533 | 0.01016677284 |
| 115.94724 | -28.46585679 | 115.9877563 | 209.7524371 | 0.008803670487 | -16.83253502 | 0.009375536182 | 2 | 2 | -150.0915287 | 0.009635973318 | -17.04297252 | 0.008771323745 |
| 114.58483 | -29.61592917 | 114.5130252 | 216.0231438 | 0.008170528535 | -12.25148893 | 0.00910110486 | 2 | 1 | -144.2399435 | 0.008162793568 | -12.69836883 | 0.007848825779 |
| 126.42504 | -32.12481642 | 126.4552174 | 204.4700957 | 0.0120139184 | -17.7466944 | 0.01415305672 | 2 | 2 | -155.1753553 | 0.01143723282 | -18.43380695 | 0.01180738016 |
| 132.53957 | -29.57883059 | 132.3571056 | 276.6414884 | 0.03069001267 | -49.3150326 | 0.01214030333 | 2 | 2 | -87.04428853 | 0.01465167222 | -48.50238584 | 0.009307966634 |
| 132.78491 | -30.12309578 | 133.1963492 | 304.9327554 | 0.01883516967 | -28.62866143 | 0.006298811768 | 2 | 1 | -53.06453207 | 0.004588437091 | -29.12891495 | 0.003873437666 |
| 139.72748 | -29.48200614 | 140.2908267 | 317.2221123 | 0.05654086996 | -17.86041368 | 0.02884410581 | 3 | 2 | -38.37281546 | 0.01069679734 | -19.7141681 | 0.009857816208 |
| 137.50014 | -32.353744 | 137.7435882 | 344.9634576 | 0.008639902079 | 0.8232895088 | 0.01230609365 | 2 | 2 | -14.41704408 | 0.01005770259 | 0.09496991099 | 0.01034106493 |
| 139.76145 | -29.48027428 | 140.2980241 | 315.8884391 | 0.05471541891 | -17.69867547 | 0.02515078043 | 3 | 3 | -39.59110314 | 0.007107122729 | -19.61710823 | 0.006248532754 |
| 140.68674 | -29.90287992 | 140.9065628 | 248.7464807 | 0.1710218004 | -25.29108896 | 0.0496988975 | 3 | 1 | -103.470784 | 0.005653420871 | -27.22393157 | 0.004750768307 |
| 124.43451 | -30.99187464 | 124.4709441 | 317.1389918 | 0.01380646478 | 18.30126453 | 0.04129242348 | 3 | 1 | -42.5280227 | 0.01076207568 | 14.42348331 | 0.01111442717 |
| 133.27540 | -30.79274609 | 133.423048 | 7.539050347 | 0.01384062722 | -1.678199064 | 0.01638295738 | 2 | 2 | 8.040643596 | 0.01454939706 | -2.435313554 | 0.01575562318 |
| 133.71820 | -28.96935339 | 134.1395495 | 45.30314571 | 0.02125089507 | 0.3522579515 | 0.02064391305 | 3 | 3 | 46.53014926 | 0.01855988643 | -0.5737874533 | 0.01818066685 |
| 137.47141 | -31.11589824 | 137.5438743 | 99.53698546 | 0.0164177076 | -53.148007 | 0.006939592797 | 2 | 1 | 100.6831582 | 0.01372715461 | -52.45168042 | 0.007808713917 |
| 131.64999 | -31.13440653 | 131.8370961 | 184.3947845 | 0.01126327203 | 0.7263270409 | 0.01147140197 | 2 | 2 | -174.9622717 | 0.0109789817 | -0.04450068015 | 0.0108936652 |
| 135.34589 | -30.75836984 | 135.1678381 | 184.5865441 | 0.01665584732 | -32.38771662 | 0.009842350169 | 2 | 2 | -177.3508726 | 0.01084057225 | -32.58188676 | 0.008368813649 |
| 128.36587 | -31.58028419 | 128.1810362 | 223.5137633 | 0.01765220377 | -26.89724265 | 0.01137052242 | 5 | 5 | -137.4737764 | 0.0135056247 | -27.16362895 | 0.01203122076 |
| 139.23398 | -32.75092882 | 139.8280444 | 239.3814309 | 0.02342843313 | -27.08630437 | 0.01618011815 | 3 | 3 | -119.0292303 | 0.01890919696 | -27.65967491 | 0.01559647525 |
| 126.64032 | -30.2921535 | 126.2422497 | 247.1571978 | 0.008969240007 | -13.16402486 | 0.009805012607 | 4 | 3 | -113.9013662 | 0.008270929703 | -13.72159838 | 0.007840183654 |
| 126.21926 | -29.72406935 | 126.2988246 | 255.7189347 | 0.01023243209 | -14.80995269 | 0.01353844795 | 4 | 4 | -104.0386726 | 0.01364346826 | -15.12006008 | 0.01404185548 |
| 131.07564 | -31.58932738 | 130.8671258 | 252.6211696 | 0.01252364887 | -14.4676019 | 0.01338355463 | 5 | 5 | -107.8543545 | 0.01209143269 | -14.89351597 | 0.01231123702 |
| 126.24598 | -32.35784321 | 126.498293 | 254.3912003 | 0.01427640893 | -14.08606356 | 0.01070811368 | 2 | 2 | -104.6591368 | 0.01128462722 | -14.68279186 | 0.01043578581 |
| 136.06761 | -29.72227161 | 136.2351972 | 257.8547399 | 0.01522868482 | -15.03701528 | 0.01549658424 | 3 | 3 | -101.568148 | 0.01355827253 | -15.4263871 | 0.01324026023 |
| 116.31617 | -29.3927055 | 116.3618078 | 315.3921448 | 0.009611272837 | -27.08621317 | 0.006979822643 | 2 | 2 | -44.35300331 | 0.008058573875 | -27.1377109 | 0.007020881994 |
| 138.68267 | -26.41294461 | 138.2858942 | 306.8739369 | 0.01361689047 | -18.01856919 | 0.01153869351 | 3 | 2 | -54.85828937 | 0.01176971878 | -18.59332319 | 0.01067992096 |
| 131.71533 | -32.36752938 | 131.6664874 | 323.2908252 | 0.009110470714 | -13.4971418 | 0.009103072336 | 2 | 2 | -36.8766433 | 0.00844853516 | -13.97239658 | 0.008392488768 |
| 137.42532 | -31.78250744 | 137.0937612 | 328.1444316 | 0.01367548695 | -2.950443702 | 0.01532214068 | 3 | 2 | -33.04723807 | 0.0139270444 | -4.052495996 | 0.01403270686 |
| 136.68589 | -31.18355562 | 136.9158399 | 352.3208334 | 0.01124471341 | -18.18228808 | 0.009600351049 | 2 | 2 | -7.111100248 | 0.008945134092 | -18.54557041 | 0.008549861614 |
| 132.39432 | -31.41467056 | 131.9752372 | 359.4556244 | 0.01150381278 | -10.44785936 | 0.01007595461 | 2 | 2 | -2.200223083 | 0.008572542716 | -11.39949036 | 0.008412507903 |
| 115.20765 | -30.11752907 | 115.0226096 | 112.9868889 | 0.01453691551 | -40.5207148 | 0.01149699206 | 2 | 2 | 112.0850667 | 0.0137355412 | -40.5138705 | 0.009763657597 |
| 138.40875 | -29.32734591 | 138.2598125 | 355.4103122 | 0.02243290185 | 12.15188662 | 0.05697230944 | 13 | 9 | -6.422086921 | 0.0164286305 | 7.27115074 | 0.01742088811 |
| 118.96753 | -32.07509888 | 118.9192532 | 92.06875389 | 0.01387182668 | -36.10041478 | 0.0105595217 | 4 | 1 | 91.93144336 | 0.0125961 | -36.02022191 | 0.009964005906 |
| 127.19574 | -30.61967272 | 127.1121049 | 136.2498691 | 0.02151366543 | -48.43838451 | 0.01142902071 | 2 | 2 | 135.8624665 | 0.02018359197 | -48.17693353 | 0.01273986846 |
| 137.58434 | -30.43275758 | 137.3791829 | 123.108429 | 0.03679961354 | -44.13223959 | 0.02052507163 | 9 | 7 | 123.0577825 | 0.03728050055 | -43.84013968 | 0.02741849436 |
| 137.01459 | -30.36871066 | 136.9266342 | 227.7376729 | 0.009160801355 | -20.68846511 | 0.009075368596 | 3 | 3 | -132.6920983 | 0.00840442778 | -20.98009608 | 0.008007266998 |
| 141.07112 | -31.71105616 | 140.9525045 | 249.4415905 | 0.01146236534 | -32.21998758 | 0.008913130507 | 2 | 1 | -111.6665713 | 0.009293042359 | -32.28129526 | 0.007766412448 |
| 129.47883 | -31.60265258 | 129.7778305 | 330.6409807 | 0.00911754499 | -6.857592705 | 0.008887101333 | 2 | 2 | -28.58796227 | 0.008092810913 | -7.500820526 | 0.008263247413 |
| 141.42237 | -33.47923254 | 140.8609898 | 354.1065805 | 0.01167921749 | 4.978778032 | 0.01161939608 | 2 | 1 | -7.10025853 | 0.01124335071 | 4.004154898 | 0.01184132899 |
| 118.83992 | -28.45863664 | 118.4033772 | 208.2724359 | 0.00924697596 | -16.56919726 | 0.004826804754 | 2 | 1 | -153.2535979 | 0.003946047244 | -17.19425667 | 0.00342332277 |
| -121.62986 | 40.48450242 | -122.6757138 | 31.32045495 | 0.01357697501 | 16.65298377 | 0.01110450616 | 2 | 1 | 29.30857583 | 0.006539676297 | 18.10132388 | 0.006833323492 |
| 42.83560 | 26.7425807 | 42.59334111 | 101.1098149 | 0.003982102995 | 14.33317448 | 0.004410401143 | 2 | 2 | 100.6144517 | 0.004287949156 | 14.62732903 | 0.004058428238 |
| 114.75483 | -30.41171418 | 114.4938272 | 97.523839 | 0.01536338524 | 0.8133917256 | 0.01532150746 | 2 | 2 | 96.86766639 | 0.01452833441 | -0.2606328054 | 0.01309199452 |
| 128.98799 | -29.14351521 | 129.1665954 | 204.9673344 | 0.009741483683 | 7.235181438 | 0.01136181947 | 3 | 1 | 26.19752928 | 0.00852189297 | -6.058880169 | 0.009075220464 |
| 119.54203 | -34.4686199 | 119.6053512 | 224.7142334 | 0.007912019485 | -17.73617503 | 0.007873670891 | 3 | 3 | -134.9420333 | 0.006316752958 | -18.42108 | 0.006083111976 |
| -0.64264 | 51.39446976 | -1.409972119 | 234.4314039 | 0.0103960607 | -15.62927806 | 0.02023711805 | 2 | 2 | -127.0658109 | 0.00869657202 | -12.57926004 | 0.008567716923 |

# Table A3

| initial_v | initial_v_err | final_v | final_v_err | initial_height | final_height | peak_brightness_height | semi_major_axis | err_semi_major_axis | eccentricity | err_eccentricity | inclination | err_inclination |
|---|---|---|---|---|---|---|---|---|---|---|---|---|
| 18357.04834 | 90.51469238 | 14021.10914 | 168.7769998 | 81697.34778 | 48272.02238 | 58783.5267 | 3.001718959 | 0.05107625528 | 0.6760088337 | 0.005508545871 | 17.3614965 | 0.1204699895 |
| 44658.78158 | 89.79363485 | 42812.02 | 56.838 | 93280.02998 | 66006.7765 | 77204.96985 | 2.518944325 | 0.04139333638 | 0.6090697029 | 0.006463940911 | 77.02931605 | 0.1016375873 |
| 20849.59242 | 94.02121294 | 18062.31 | 81.7796 | 77641.87749 | 58032.65684 | 71997.90773 | 2.914887521 | 0.06233994082 | 0.7242083701 | 0.006164890244 | 11.71749728 | 0.08238064421 |
| 38009.4326 | 133.8781063 | 33635.85264 | 299.9820501 | 80383.29487 | 45489.06966 | 53390.76077 | 2.24257449 | 0.03867315668 | 0.9295610325 | 0.001729939717 | 0.530424802 | 0.01722912665 |
| 28419.34918 | 110.7118697 | 16883.859 | 65.6439 | 81666.36371 | 38537.35846 | 51408.97919 | 2.594892622 | 0.03807085379 | 0.8180909017 | 0.003276270991 | 2.012048552 | 0.01133182938 |
| 38868.70486 | 93.52164743 | 26862.367 | 59.771 | 96402.69486 | 44309.62033 | 49658.84456 | 2.424209964 | 0.02887557588 | 0.9398155063 | 0.001022530862 | 12.74384434 | 0.06272196155 |
| 41608.66611 | 101.1562782 | 38000.697 | 60.221 | 93093.79867 | 61922.99557 | 79913.37627 | 2.487778774 | 0.04798248413 | 0.9630770345 | 0.001040916697 | 14.08323501 | 0.1087960168 |
| 35325.88039 | 113.7483195 | 30328.694 | 72.69 | 82210.08187 | 49149.58278 | 54211.69624 | 2.441023526 | 0.04042465809 | 0.8996425453 | 0.002122183633 | 3.205858659 | 0.01844915408 |
| 26042.0725 | 99.34268102 | 21276.121 | 74.463 | 79523.78516 | 51919.536 | 65151.02201 | 2.684382819 | 0.03697746236 | 0.7836853476 | 0.003357346487 | 5.506957915 | 0.02744186519 |
| 22284.77276 | 87.55839954 | 18192.602 | 66.515 | 90795.60015 | 55849.37718 | 58835.19174 | 3.394467654 | 0.07016960934 | 0.7654886933 | 0.004952601697 | 13.96724031 | 0.05273406512 |
| 29697.86098 | 108.2099427 | 16709.683 | 69.538 | 86047.31181 | 45772.07847 | 58340.03887 | 2.516658483 | 0.03600968127 | 0.8360487742 | 0.002896267732 | 9.632969506 | 0.05833085722 |
| 22020.08336 | 92.94767339 | 14656.992 | 74.438 | 79029.85608 | 44892.7576 | 58655.99005 | 2.800106659 | 0.05077988087 | 0.751225397 | 0.00507431517 | 0.8270018126 | 0.03100560216 |
| 39370.24461 | 90.96494766 | 35231.821 | 56.442 | 95455.04024 | 63502.49892 | 78438.16167 | 3.047546955 | 0.05548144926 | 0.9547814631 | 0.001051684224 | 16.85297852 | 0.07062772038 |
| 21928.27074 | 127.9915352 | 12999.78 | 147.514 | 76703.46279 | 45024.41884 | 58803.63307 | 2.983154658 | 0.05709153637 | 0.7625743907 | 0.005055973211 | 0.5072973943 | 0.02604463364 |
| 14535.19535 | 98.3918335 | 11651.747 | 96.535 | 87190.98034 | 53381.76717 | 64060.51361 | 3.592275469 | 0.1678287994 | 0.7197016042 | 0.01284517594 | 0.8100322895 | 0.01680804679 |
| 20973.26884 | 89.06168661 | 5936.146965 | 108.8196061 | 86354.95196 | 33437.94804 | 48914.48639 | 2.87901556 | 0.05124657449 | 0.7132513156 | 0.005356468304 | 16.05352462 | 0.0606632536 |
| 35507.50972 | 85.33062535 | 25669.092 | 55.297 | 96404.96318 | 61301.13628 | 87346.84808 | 2.300437665 | 0.02223605072 | 0.9122523787 | 0.001098528866 | 8.372962503 | 0.04987783056 |
| 33947.71536 | 119.0138656 | 28402.108 | 60.052 | 96916.81317 | 59799.00017 | 70541.90371 | 3.011254102 | 0.05392126908 | 0.8907600638 | 0.002235420482 | 22.3337215 | 0.1072925606 |
| 30036.65927 | 85.53550262 | 22967.093 | 62.284 | 90323.85135 | 59662.37821 |  | 2.591101183 | 0.02675384733 | 0.6311651236 | 0.00379863492 | 45.98008907 | 0.09333340276 |
| 37227.96693 | 118.0454637 | 36489.1325 | 114.0925429 | 97128.33449 | 68728.27126 | 82365.22287 | 2.311792525 | 0.04049447569 | 0.9219110354 | 0.001898068014 | 4.881562005 | 0.03622359146 |
| 25947.20694 | 102.4037303 | 22335.598 | 69.851 | 90216.07335 | 61951.08907 | 70449.0791 | 2.679897642 | 0.05067939303 | 0.749399043 | 0.005055740157 | 19.54444375 | 0.1009797158 |
| 29640.99855 | 97.81916929 | 26127.787 | 63.946 | 84540.19068 | 50945.10231 | 63873.606 | 2.535004716 | 0.03197711636 | 0.8209206309 | 0.002567245909 | 9.988659358 | 0.04013615953 |
| 34816.56225 | 103.2394075 | 25657.005 | 60.331 | 90231.78414 | 47707.07004 | 53429.0429 | 2.31236211 | 0.03301321338 | 0.8949432255 | 0.001972354414 | 10.84927798 | 0.07220016297 |
| 37732.89994 | 97.11659702 | 33708.853 | 60.65 | 90343.45474 | 55606.21552 | 65175.72537 | 2.463330555 | 0.03579336325 | 0.9210807103 | 0.001458355072 | 17.05828203 | 0.07366787687 |
| 39235.85915 | 91.7399788 | 34273.832 | 57.028 | 85120.8043 | 47652.55627 | 55218.23284 | 2.327548668 | 0.03154651997 | 0.9403821689 | 0.001091835551 | 19.91100713 | 0.1126551469 |
| 37221.10486 | 101.6007643 | 26725.203 | 56.707 | 93655.7027 | 47670.18914 | 66727.60105 | 2.420730124 | 0.03466326505 | 0.9179196562 | 0.001520301858 | 15.59247952 | 0.07249829028 |
| 35022.60062 | 108.8371934 | 29034.761 | 72.164 | 82088.7912 | 51824.08085 | 60526.12089 | 2.352824966 | 0.03298393289 | 0.8961562531 | 0.001930393374 | 14.35490928 | 0.07216945472 |
| 36439.13598 | 93.62553284 | 33249.419 | 52.752 | 96776.26267 | 60902.94852 | 68838.60194 | 2.247396202 | 0.02521924105 | 0.911348534 | 0.001346584661 | 15.30671514 | 0.06895412204 |
| 43223.80664 | 203.5761057 | 42458.47293 | 197.2584797 | 83192.69501 | 62942.57713 |  | 2.596992101 | 0.08275227136 | 0.9710679651 | 0.001223846365 | 38.89757194 | 0.460127352 |
| 29182.39309 | 95.8057332 | 15166.805 | 76.204 | 82574.88425 | 38567.42831 | 48664.30869 | 2.695299699 | 0.03968758045 | 0.8336386157 | 0.002773386272 | 1.078348193 | 0.01374651789 |
| 35812.71579 | 108.1826664 | 31245.446 | 68.892 | 80452.1065 | 47651.43315 | 53638.00274 | 2.338769298 | 0.03182693633 | 0.9149144349 | 0.001548740237 | 1.83425069 | 0.01662884945 |
| 31097.24356 | 88.33776853 | 27064.878 | 64.612 | 90537.14609 | 54482.51468 | 59125.17939 | 2.430173306 | 0.03440582302 | 0.8473151926 | 0.002525010767 | 11.08766322 | 0.0419358762 |
| 35862.63737 | 126.0407346 | 9922.812 | 67.606 | 90125.29649 | 37986.29749 | 57541.82745 | 2.519007403 | 0.04082409173 | 0.9044903125 | 0.001877232821 | 23.92640975 | 0.1296929801 |
| 32889.2659 | 99.44720426 | 29179.888 | 68.822 | 85389.93924 | 58529.84842 | 63817.82432 | 2.471387534 | 0.0336244763 | 0.8718990208 | 0.002027812796 | 12.6486857 | 0.05217277201 |
| 43433.17687 | 118.893747 | 42025.33796 | 159.1855445 | 85956.69867 | 60754.67777 | 75920.69865 | 2.506646468 | 0.05566903465 | 0.6036804327 | 0.008735346773 | 75.03329745 | 0.1486918273 |
| 17599.02909 | 87.58445438 | 15516.51411 | 121.6332703 | 91810.21499 | 53627.14418 | 58842.64613 | 3.60775747 | 0.08704061878 | 0.7512051867 | 0.006068230426 | 4.62925313 | 0.01087796305 |
| 39202.44639 | 103.4045284 | 30266.764 | 65.43 | 87274.49127 | 45524.7411 | 56193.0202 | 2.835599975 | 0.05606440844 | 0.7011323133 | 0.00572540286 | 63.75061755 | 0.1341913959 |
| 44241.92444 | 99.68061989 | 41453.158 | 57.465 | 100093.3373 | 65771.75178 | 79681.2937 | 2.797430375 | 0.04502917991 | 0.651236897 | 0.005608885368 | 75.74692962 | 0.09381083435 |
| 43138.62951 | 98.24361223 | 36073.666 | 53.721 | 101621.6981 | 41474.69007 | 63295.51626 | 2.683646577 | 0.03957719701 | 0.6393580131 | 0.005305994116 | 73.47459893 | 0.09451820871 |
| 33669.27708 | 93.19873167 | 30738.423 | 58.332 | 90939.16672 | 60555.7074 | 70281.04925 | 2.309303355 | 0.02762336059 | 0.8762522192 | 0.001881897732 | 4.090266635 | 0.02079300585 |
| 25998.35108 | 119.5722476 | 20494.99 | 68.957 | 91869.78888 | 59719.43947 |  | 2.776330936 | 0.04679070755 | 0.7866991294 | 0.003970517824 | 7.735961588 | 0.03483731614 |
| 37223.82687 | 90.51683894 | 27386.98 | 67.287 | 82976.39082 | 44975.74329 |  | 2.411890487 | 0.03063286569 | 0.9328643587 | 0.001182115986 | 10.55964801 | 0.04490185302 |
| 39856.08419 | 109.6473362 | 39165.91244 | 108.2081703 | 95836.07989 | 72026.28474 | 81780.4177 | 2.63744778 | 0.05808214767 | 0.9516801372 | 0.00137601751 | 18.09606376 | 0.1202382047 |
| 35487.4953 | 99.52824 | 32526.74494 | 201.8430187 | 75509.2737 | 46297.32001 |  | 2.360762993 | 0.03379306154 | 0.894927043 | 0.001869023153 | 7.613478783 | 0.04370791614 |
| 29772.39629 | 88.09256693 | 8212.15 | 68.468 | 88198.67597 | 32791.48565 |  | 2.44232961 | 0.03022677549 | 0.83316696 | 0.002411542161 | 3.929985867 | 0.02835988934 |
| 38887.84928 | 93.5437893 | 23061.071 | 63.136 | 98910.96026 | 47826.61782 |  | 2.522537594 | 0.03646223114 | 0.9348349907 | 0.001210742155 | 19.16560666 | 0.08516211574 |
| 31207.69874 | 85.75510218 | 12922.802 | 62.411 | 90757.03583 | 34694.14482 |  | 4.283263377 | 0.1022587901 | 0.8807469982 | 0.002956668991 | 21.88284046 | 0.07510188147 |
| 31475.96776 | 91.23802764 | 16715.936 | 81.045 | 88465.07819 | 41970.34631 |  | 2.628841722 | 0.03450542533 | 0.8406747791 | 0.002431261257 | 18.59175338 | 0.06651615285 |
| 28087.62662 | 88.60189623 | 21557.943 | 70.573 | 80041.77416 | 40062.77055 |  | 2.564944128 | 0.03357431262 | 0.8099047508 | 0.002932514885 | 0.6932912647 | 0.008382253951 |
| 28977.55425 | 76.78138245 | 26111.663 | 69.857 | 90845.6727 | 65979.682 |  | 2.728328467 | 0.03711452609 | 0.825936712 | 0.002627878888 | 3.566882666 | 0.02878429742 |

# Table A4

| argument_periapsis | err_argument_periapsis | longitude_ascending_node | err_longitude_ascending_node | perihelion | err_perihelion | aphelion | err_aphelion | Tj | err_Tj | m0 | m0_err |
|---|---|---|---|---|---|---|---|---|---|---|---|
| 337.6495176 | 0.06403789723 | 3.336283681 | 2.75E-04 | 0.9722491319 | 3.51E-05 | 5.031188785 | 0.1021308898 | 2.80184368 | 0.01542255254 | 0.4062258231 | 0.1495070175 |
| 359.3802588 | 0.0578251217 | 81.24816209 | 9.10E-06 | 0.9844641658 | 4.00E-06 | 4.053424484 | 0.08278551199 | 2.313410604 | 0.01283037734 | 0.1116597336 | 0.02273110721 |
| 55.62903491 | 0.02268540967 | 111.8172577 | 2.15E-04 | 0.8035173492 | 7.78E-04 | 5.026257693 | 0.1254536974 | 2.79583635 | 0.01954390024 | 0.01519402133 | 0.001816112686 |
| 138.1222418 | 0.07037196501 | 170.726113 | 0.003650429398 | 0.1578978003 | 0.001178032976 | 4.327251181 | 0.07851527147 | 2.804300122 | 0.01664033783 | 0.714078862 | 0.1083578862 |
| 279.8149986 | 0.0554953605 | 3.643798842 | 2.14E-05 | 0.4719099176 | 0.001561677029 | 4.717875327 | 0.07769052133 | 2.816968475 | 0.0139867596 | 1.312572208 | 0.2907641793 |
| 319.6452674 | 0.0528321142 | 3.635076776 | 8.32E-06 | 0.1458703754 | 7.55E-04 | 4.702549552 | 0.05849351348 | 2.601365482 | 0.01069394862 | 0.7704496831 | 0.1267206586 |
| 148.3057125 | 0.07255132774 | 187.5478457 | 2.42E-06 | 0.09180629089 | 8.19E-04 | 4.883751257 | 0.09677714902 | 2.452694443 | 0.01630368048 | 0.02700149428 | 0.002625243269 |
| 306.5550972 | 0.03283108399 | 21.26459602 | 2.36E-05 | 0.244889188 | 0.001128445771 | 4.637157864 | 0.08196683333 | 2.729288572 | 0.01541252477 | 0.1827729187 | 0.0239161435 |
| 87.7624317 | 0.02239031036 | 210.0383623 | 4.98E-05 | 0.5805472291 | 0.001088284164 | 4.788218409 | 0.0750286924 | 2.826567778 | 0.01296666802 | 0.04801367814 | 0.00554713357 |
| 60.08796687 | 0.04242765773 | 289.605319 | 2.26E-05 | 0.7956937131 | 5.53E-04 | 5.993241594 | 0.140883624 | 2.541576729 | 0.01715644427 | 0.02359869393 | 0.00406220491 |
| 107.7590842 | 0.02361860607 | 291.8399472 | 9.17E-06 | 0.4125049906 | 0.001308635292 | 4.620811975 | 0.07332456364 | 2.819939698 | 0.0136961152 | 0.2144041766 | 0.03400879862 |
| 74.18478395 | 0.07199271509 | 323.4236165 | 0.001757231761 | 0.696337853 | 0.001716464152 | 4.903875465 | 0.1032674364 | 2.826559972 | 0.01698693446 | 0.2427840508 | 0.04729344655 |
| 320.2539289 | 0.04455521921 | 143.3597201 | 6.11E-06 | 0.1377473413 | 7.24E-04 | 5.957346568 | 0.1116756352 | 2.142911723 | 0.01336066715 | 0.02619075355 | 0.003194622195 |
| 72.1962096 | 0.07267636248 | 323.4506273 | 0.00379646324 | 0.7079887815 | 0.001642479329 | 5.258320534 | 0.1158209878 | 2.723842912 | 0.01726237636 | 0.224 | 0.04166750307 |
| 11.02689788 | 0.09387321996 | 324.0799989 | 0.001113155721 | 1.004756565 | 2.14E-04 | 6.179794373 | 0.3358717376 | 2.602115729 | 0.03891894893 | 0.01163393619 | 0.002279698429 |
| 235.6685343 | 0.0268920742 | 162.4926331 | 6.09E-05 | 0.8252795157 | 6.79E-04 | 4.932751604 | 0.1031649424 | 2.809406966 | 0.01634644688 | 0.563454361 | 0.1267553278 |
| 132.5357158 | 0.03097600538 | 346.5280935 | 5.48E-05 | 0.2018336054 | 6.11E-04 | 4.399041724 | 0.04504054714 | 2.800827812 | 0.009241718163 | 0.02049042481 | 0.002572693892 |
| 114.9183427 | 0.04857888323 | 27.86503264 | 5.65E-05 | 0.3288289477 | 8.53E-04 | 5.693679257 | 0.1086009508 | 2.367568215 | 0.01436186836 | 0.04404270234 | 0.009528970697 |
| 22.59122011 | 0.05346799634 | 78.1257327 | 2.22E-05 | 0.9555868656 | 4.11E-05 | 4.2266155 | 0.05348294891 | 2.768882706 | 0.009446088233 | 0.02012738333 | 0.002414853071 |
| 314.8704052 | 0.06559976604 | 343.3903049 | 1.02E-04 | 0.1804487069 | 0.001242756802 | 4.443136344 | 0.08222138843 | 2.765362946 | 0.01665100389 | 0.01245024449 | 0.002182853122 |
| 76.70427951 | 0.06765370853 | 199.8265585 | 9.06E-05 | 0.6713287971 | 8.08E-04 | 4.688466487 | 0.1021556288 | 2.837218994 | 0.01773733368 | 0.01136896715 | 0.001551154323 |
| 102.6776966 | 0.03806177587 | 222.3443291 | 3.72E-06 | 0.4538850437 | 8.02E-04 | 4.616124388 | 0.06471240753 | 2.837681788 | 0.01199003284 | 0.1384495971 | 0.02193041027 |
| 127.4273238 | 0.05769340697 | 225.5158314 | 3.65E-05 | 0.2428644125 | 0.001188204869 | 4.381859807 | 0.06715884752 | 2.834479507 | 0.01385104144 | 0.3821931879 | 0.06232687632 |
| 313.1582932 | 0.02254251773 | 47.2013821 | 1.79E-05 | 0.1943521624 | 7.58E-04 | 4.732308947 | 0.07233011528 | 2.624569769 | 0.01301982076 | 0.1361859563 | 0.01848917254 |
| 321.2656412 | 0.03621453093 | 52.21676796 | 3.14E-05 | 0.1387290437 | 6.84E-04 | 4.516368291 | 0.06375680172 | 2.663314596 | 0.01238427104 | 0.3605356913 | 0.04104473222 |
| 312.7410982 | 0.03131812481 | 53.06068265 | 2.78E-05 | 0.19864178 | 8.33E-04 | 4.642818468 | 0.07013441654 | 2.670829929 | 0.01307691817 | 0.2687453591 | 0.03726906388 |
| 307.2181633 | 0.04239138256 | 57.0967007 | 3.44E-05 | 0.2442625559 | 0.001126019092 | 4.461387377 | 0.06707907172 | 2.789680485 | 0.01341117114 | 0.1289617234 | 0.01482716438 |
| 313.1770415 | 0.04567442666 | 58.00134802 | 3.06E-05 | 0.1992011609 | 8.42E-04 | 4.295591243 | 0.05123268022 | 2.837146101 | 0.01092638658 | 0.02688613278 | 0.00333879907 |
| 151.6446237 | 0.05051185269 | 280.1480545 | 2.59E-05 | 0.07503518651 | 8.03E-04 | 5.118949016 | 0.1663017415 | 2.26621079 | 0.02478772983 | 0.02630363908 | 0.002820150296 |
| 283.1642678 | 0.0269601836 | 119.0081071 | 0.001030283563 | 0.4482837876 | 9.15E-04 | 4.94231561 | 0.08026915798 | 2.725405134 | 0.01343649492 | 0.7498617642 | 0.1221260416 |
| 313.0514215 | 0.0367692251 | 121.9815466 | 3.04E-04 | 0.1989462777 | 9.22E-04 | 4.478592318 | 0.06456162451 | 2.765785194 | 0.01288980153 | 0.2592230476 | 0.02870098647 |
| 292.4718021 | 0.03161187394 | 138.0926203 | 6.28E-05 | 0.370963754 | 9.33E-04 | 4.489382857 | 0.06971436858 | 2.853496368 | 0.01360531412 | 0.07060594139 | 0.01028675222 |
| 127.243035 | 0.02006923217 | 325.9908487 | 1.31E-05 | 0.2405130365 | 8.29E-04 | 4.797501769 | 0.08246159142 | 2.608132842 | 0.01440487971 | 1.068061706 | 0.1577821057 |
| 118.2418132 | 0.02628199773 | 341.198207 | 7.20E-06 | 0.3165190464 | 7.33E-04 | 4.626256022 | 0.06796455826 | 2.764017983 | 0.01268454757 | 0.06283425739 | 0.008438235124 |
| 355.8777312 | 0.0462800904 | 33.53738756 | 1.31E-05 | 0.9929470206 | 1.62E-05 | 4.020345916 | 0.1113304872 | 2.361631127 | 0.01768063377 | 0.06040028087 | 0.005643462553 |
| 219.3341747 | 0.02694048525 | 215.1967063 | 1.06E-04 | 0.8970634623 | 3.51E-04 | 6.318451478 | 0.1744231319 | 2.537933007 | 0.01982985489 | 0.02575282656 | 0.00692277716 |
| 49.58959981 | 0.2163363385 | 45.56150854 | 1.56E-05 | 0.8471483423 | 4.99E-04 | 4.824051607 | 0.1116535185 | 2.300615548 | 0.01522408217 | 0.4608656117 | 0.06677470301 |
| 346.085882 | 0.07907673403 | 64.72984163 | 9.35E-06 | 0.9753879796 | 8.47E-05 | 4.61947277 | 0.09000790349 | 2.134041007 | 0.01159067348 | 0.0212232717 | 0.002284428944 |
| 17.92894248 | 0.1039561572 | 67.67770017 | 9.91E-06 | 0.9676256789 | 1.52E-04 | 4.399667475 | 0.07907750843 | 2.253050574 | 0.01119720716 | 1.684254273 | 0.3376665164 |
| 122.2476874 | 0.02566409418 | 216.3021921 | 5.74E-05 | 0.2857192382 | 9.47E-04 | 4.332887472 | 0.05617686258 | 2.893593771 | 0.01178115173 | 0.02244575213 | 0.002569578795 |
| 86.91028872 | 0.02591865515 | 253.845206 | 6.68E-05 | 0.5920080714 | 0.001053397026 | 4.960653801 | 0.09462454712 | 2.767852242 | 0.01549450429 | 0.01135774897 | 0.001881434904 |
| 317.8586801 | 0.04457752716 | 128.5273216 | 7.99E-06 | 0.1618876598 | 8.02E-04 | 4.661893314 | 0.06205589569 | 2.639870487 | 0.01153342931 | 0.5403769861 | 0.06484477151 |
| 322.4066123 | 0.04200251956 | 152.2367665 | 9.19E-06 | 0.1273612956 | 8.52E-04 | 5.147534264 | 0.1170043703 | 2.388516929 | 0.01798175973 | 0.0126526864 | 0.001852948133 |
| 126.3322485 | 0.009881963712 | 195.4490453 | 4.58E-05 | 0.24798922 | 8.56E-04 | 4.473536766 | 0.06843838894 | 2.800290719 | 0.01361864991 | 2.105720489 | 0.4263253851 |
| 287.4616063 | 0.01841899462 | 206.209909 | 9.45E-05 | 0.4073884091 | 8.37E-04 | 4.477270811 | 0.06128214968 | 2.886729148 | 0.0120097168 | 3.255584855 | 0.6830295399 |
| 136.4048892 | 0.02513902467 | 78.23380663 | 3.54E-05 | 0.1643370651 | 6.86E-04 | 4.880738122 | 0.07360684772 | 2.530174489 | 0.01250344501 | 0.2869341025 | 0.03809599283 |
| 91.54137267 | 0.05026567403 | 92.24525071 | 5.69E-05 | 0.5104899054 | 5.72E-04 | 8.056036848 | 0.2050310084 | 2.012706631 | 0.01599804147 | 1.292364446 | 0.2018203494 |
| 285.7643088 | 0.02051860216 | 10.21515271 | 9.89E-06 | 0.4187569522 | 9.15E-04 | 4.838926492 | 0.0699074712 | 2.709269068 | 0.01200030671 | 0.5088291976 | 0.07268292404 |
| 98.96922138 | 0.01625502521 | 223.3444939 | 0.001106237939 | 0.4874852735 | 0.00112731783 | 4.642402982 | 0.06826915972 | 2.85223105 | 0.01254494019 | 0.593400439 | 0.07561027467 |
| 279.818645 | 0.03112825781 | 51.42940855 | 5.69E-04 | 0.4748043262 | 7.28E-04 | 4.981852608 | 0.07494456939 | 2.722035769 | 0.01235600708 | 0.03413005015 | 0.005664060852 |

# Table A5

| ballistic_alpha | ballistic_beta | ram_pressure_i | ram_pressure_f | ram_pressure_pb | atm_density_initial | atm_density_final | PE | PE_err |
|---|---|---|---|---|---|---|---|---|
| 132.2637854 | 2.636136972 | 4563.216645 | 263861.9946 | 111382.0075 | 1.35E-05 | 0.001342184137 | -4.276730967 | 0.08937218026 |
| 187.08194 | 1.00E-04 | 4645.726064 | 289296.4275 | 62091.7361 | 2.33E-06 | 1.58E-04 | -4.834848875 | 0.03822916543 |
| 391.3875519 | 0.5074018699 | 12394.13924 | 144186.9282 | 30733.62867 | 2.85E-05 | 4.42E-04 | -4.790052552 | 0.02337465956 |
| 62.96900806 | 0.3338185835 | 24091.52384 | 2180934.497 | 978780.9238 | 1.67E-05 | 0.00192769242 | -4.499070848 | 0.02966383782 |
| 58.7661082 | 1.417831671 | 10933.97131 | 1405186.432 | 590352.3096 | 1.35E-05 | 0.004929359749 | -4.110493487 | 0.04332047982 |
| 119.5987066 | 1.459771964 | 2066.19227 | 1603884.464 | 1216108.362 | 1.37E-06 | 0.002222718807 | -4.251051982 | 0.03174912497 |
| 588.4403599 | 5.602521472 | 3995.492651 | 352495.2819 | 29628.28423 | 2.31E-06 | 2.44E-04 | -4.785894511 | 0.01806319784 |
| 57.13783683 | 10 | 15524.3708 | 1081279.995 | 732343.0897 | 1.24E-05 | 0.001175521968 | -4.538362455 | 0.02412156692 |
| 310.0448 | 1.00E-04 | 12367.09646 | 373691.9617 | 105650.4646 | 1.82E-05 | 8.26E-04 | -4.661628524 | 0.02134853922 |
| 290.0298498 | 3.441979604 | 1358.56966 | 152860.8834 | 125002.3112 | 2.74E-06 | 4.62E-04 | -4.792770601 | 0.03200534527 |
| 175.8452521 | 1.820170685 | 5644.984101 | 480103.8718 | 274931.0105 | 6.40E-06 | 0.001719486563 | -4.349265425 | 0.03001557765 |
| 129.0722142 | 1.570424699 | 9372.549488 | 430646.8558 | 158212.8186 | 1.93E-05 | 0.002004617785 | -4.336541539 | 0.03917560859 |
| 608.0324064 | 0.2308794347 | 1925.008912 | 231187.6979 | 32686.7646 | 1.24E-06 | 1.86E-04 | -4.764054608 | 0.02243553103 |
| 89.51196933 | 3.778861567 | 13065.47614 | 329988.9315 | 153324.907 | 2.72E-05 | 0.001952663317 | -4.32699 | 0.0351735 |
| 216.7255398 | 2.532190218 | 1121.442328 | 91024.57379 | 35967.91169 | 5.31E-06 | 6.70E-04 | -4.79364569 | 0.03787432136 |
| 69.78829775 | 1.109376918 | 2619.909362 | 377354.5741 | 394795.1016 | 5.96E-06 | 0.01070878821 | -3.961956108 | 0.04428260544 |
| 370.617 | 9.739 | 1516.25343 | 178095.7643 | 7081.046651 | 1.20E-06 | 2.70E-04 | -4.704193987 | 0.02309253145 |
| 568.6057697 | 1.00E-04 | 1453.468559 | 260329.9274 | 84604.37077 | 1.26E-06 | 3.23E-04 | -4.639335574 | 0.04182557509 |
| 497.3712071 | 4.187471841 | 3378.95326 | 184610.8512 | | 3.75E-06 | 3.50E-04 | -4.742699468 | 0.02301172748 |
| 663.4908126 | 1.00E-04 | 1736.981708 | 147655.2921 | 19234.17253 | 1.25E-06 | 1.11E-04 | -4.91545327 | 0.03312907996 |
| 583.3752349 | 1.00E-04 | 2305.643298 | 120007.5222 | 48836.1958 | 3.42E-06 | 2.41E-04 | -4.862566382 | 0.02673064622 |
| 106.3010212 | 0.4361175209 | 7322.21635 | 624762.3785 | 150638.2449 | 8.33E-06 | 9.15E-04 | -4.675859494 | 0.02932005675 |
| 192.0632377 | 1.070241633 | 3934.043083 | 902473.4075 | 629910.6695 | 3.25E-06 | 0.001370952779 | -4.357897992 | 0.03235991752 |
| 162.0724588 | 4.309445567 | 4728.106081 | 593804.7286 | 198775.9119 | 3.32E-06 | 5.23E-04 | -4.598821861 | 0.02535823482 |
| 71.20209441 | 2.916227285 | 12204.28477 | 1618456.969 | 766546.7683 | 7.93E-06 | 0.001377767163 | -4.531614118 | 0.02097671699 |
| 139.6966351 | 2.771429616 | 2520.489545 | 957223.9761 | 157866.6014 | 1.82E-06 | 0.001340205953 | -4.487031232 | 0.02622598565 |
| 153.3446034 | 3.241636244 | 14824.96692 | 671198.7426 | 305771.2434 | 1.21E-05 | 7.96E-04 | -4.537845716 | 0.02188254391 |
| 370.1136559 | 2.199056682 | 1344.513275 | 288332.5018 | 111878.228 | 1.01E-06 | 2.61E-04 | -4.792646006 | 0.02352389948 |
| 229.3827549 | 8.932738091 | 18845.41153 | 359662.7431 | | 1.01E-05 | 2.00E-04 | -4.845630338 | 0.01996277026 |
| 68.99245243 | 1.778035511 | 9587.477882 | 1153074.124 | 805198.8545 | 1.13E-05 | 0.005012668911 | -4.156060105 | 0.03027882108 |
| 83.19715449 | 0.2539754525 | 19257.93202 | 1305459.052 | 708746.8806 | 1.50E-05 | 0.00133717977 | -4.537880162 | 0.02068864633 |
| 232.1598522 | 4.174605245 | 3163.735594 | 420048.6992 | 267569.5626 | 3.27E-06 | 5.73E-04 | -4.595520435 | 0.02629581685 |
| 30.14601352 | 4.745925064 | 4160.905824 | 519018.2789 | 494882.8354 | 3.24E-06 | 0.005271244086 | -4.178474652 | 0.02870772081 |
| 230.2847686 | 1.451427093 | 7789.877759 | 306712.1485 | 179741.4439 | 7.20E-06 | 3.60E-04 | -4.604578511 | 0.0250932889 |
| 211.2736927 | 1.00E-04 | 13557.50713 | 521257.2448 | 68039.934 | 7.19E-06 | 2.95E-04 | -4.696053908 | 0.01753537804 |
| 229.1602678 | 1.00E-04 | 906.902931 | 171866.1609 | 101355.8767 | 2.93E-06 | 7.14E-04 | -4.732992825 | 0.05193208081 |
| 89.03273976 | 2.663098494 | 9030.271261 | 1803482.15 | 709529.889 | 5.88E-06 | 0.001968701478 | -4.445551959 | 0.02595582107 |
| 442.0700399 | 1.00E-04 | 1472.871486 | 279479.0379 | 39310.37181 | 7.52E-07 | 1.63E-04 | -4.848525115 | 0.01958161884 |
| 61.94678073 | 1.00E-04 | 1097.610299 | 4161867.495 | 338833.6517 | 5.90E-07 | 0.003198215246 | -4.364369275 | 0.03992459777 |
| 316.476 | 3.795 | 3408.95481 | 262805.2912 | 81828.77117 | 3.01E-06 | 2.78E-04 | -4.820456883 | 0.02105332883 |
| 416.9465141 | 4.770035786 | 1581.639857 | 122199.4362 | | 2.34E-06 | 2.91E-04 | -4.837610415 | 0.03193776126 |
| 94.68492135 | 2.155048111 | 14210.23831 | 1452331.552 | | 1.03E-05 | 0.001936321569 | -4.367506381 | 0.02253920923 |
| 1374.551711 | 1.315065997 | 1938.098159 | 83387.13305 | 19767.12766 | 1.22E-06 | 5.44E-05 | -4.809557584 | 0.02773124824 |
| 25.93744916 | 8.103036481 | 44989.21086 | 1799874.47 | | 3.57E-05 | 0.001701222071 | -4.530861766 | 0.03853837877 |
| 36.26088009 | 2.169496553 | 4053.408128 | 828100.2455 | | 4.57E-06 | 0.01227917437 | -3.829438957 | 0.04219573216 |
| 185.2415043 | 2.58686936 | 1254.170968 | 753143.7927 | | 8.29E-07 | 0.001416181625 | -4.447027855 | 0.02452593819 |
| 60.62229477 | 1.227006508 | 3270.755499 | 1474702.818 | | 3.36E-06 | 0.00883061864 | -4.014554541 | 0.02919777872 |
| 69.8669367 | 3.12863678 | 4749.980156 | 846839.3297 | | 4.79E-06 | 0.003030676771 | -4.287887736 | 0.02607525782 |
| 58.82420612 | 0.3428678814 | 13096.0212 | 1777301.525 | | 1.66E-05 | 0.003824251757 | -4.39728593 | 0.02390826871 |
| 578.5457609 | 3.286286369 | 2461.017168 | 108009.3149 | | 2.93E-06 | 1.58E-04 | -4.577748763 | 0.03171953855 |
